# Supplementary material for: Massively Multilingual Transfer for NER
Source: arXiv:1902.00193 source file (2019-06-05)
Supplement: Supplementary file 1 [file appendix.pdf]

## A Appendices

### A.1 Hyperparameters

We tuned the batch size and the learning rate using development sets in four languages,<sup>14</sup> and then fixed these hyperparameters for all other languages in each model. The batch size was 1 sentence in low-resource scenarios (in baseline L<sub>Sup</sub> and fine-tuning of RaRe), and to 100 sentences, in high-resource settings (H<sub>Sup</sub> and the pretraining phase of RaRe). The learning rate was set to 0.001 and 0.01 for the high-resource and low-resource baseline models, respectively, and to 0.005, 0.0005 for the pretraining and fine-tuning phase of RaRe based on development results for the four languages. For CoNLL datasets, we had to decrease the batch size of the pre-training phase from 100 to 20 (because of GPU memory issues).

### A.2 Cross-lingual Word Embeddings

We experimented with Wiki and CommonCrawl monolingual embeddings from `fastText` (Bojanowski et al., 2017). Each of the 41 languages is mapped to English embedding space using three methods from MUSE: 1) supervised with bilingual dictionaries; 2) seeding using identical character sequences; and 3) unsupervised training using adversarial learning (Lample et al., 2018). The cross-lingual mappings are evaluated by precision at  $k = 1$ . The resulting cross-lingual embeddings are then used in NER direct transfer in a leave-one-out setting for the 41 languages ( $41 \times 40$  transfers), and we report the mean  $F_1$  in Table 3. CommonCrawl doesn't perform well in bilingual induction despite having larger text corpora, and underperforms in direct transfer NER. It is also evident that using identical character strings instead of a bilingual dictionary as the seed for learning a supervised bilingual mapping barely effects the performance. This finding also applies to few-shot learning over larger ensembles: running RaRe over 40 source languages achieves an average  $F_1$  of 77.9 when using embeddings trained with a dictionary, versus 76.9 using string identity instead. For this reason we have used the string identity method in the paper (e.g., Table 4), providing greater portability to language pairs without a bilingual dictionary. Experiments with unsupervised mappings performed substantially worse than supervised methods, and so we didn't explore these further.

<sup>14</sup>Afrikaans, Arabic, Bulgarian and Bengali.

| Unsup                            |      | IdentChr | Sup       |       |           |
|----------------------------------|------|----------|-----------|-------|-----------|
| crawl                            | wiki | crawl    | wiki      | crawl | wiki      |
| word translation accuracy        |      |          |           |       |           |
| 34                               | 24   | 43       | <b>53</b> | 50    | <b>54</b> |
| average $F_1$ in direct transfer |      |          |           |       |           |
| 26                               | 21   | 37       | <b>44</b> | 39    | <b>45</b> |

**Table 3:** The effect of the choice of monolingual word embeddings (Common Crawl and Wikipedia), and their cross-lingual mapping on NER direct transfer.

### A.3 Direct Transfer Results

In Figure 5 the performance of an NER model trained in a high-resource setting on a source language applied on the other 40 target languages (leave-one-out) is shown. An interesting finding is that symmetry does not always hold (e.g. `id` vs. `ms` or `fa` vs. `ar`).

### A.4 Detailed Low-resource Results

The result of applying baselines, proposed models and their variations, and unsupervised transfer model of Xie et al. (2018) are shown in Table 4.

| Target Language | ar | he | id | ms | tl | vi | it | lv | af | da | de | en | no | sv | el | fa | bn | hi | ta | ca | es | fr | it | pt | ro | bg | mk | ru | uk | bs | cs | hr | pl | sk | sl | sq | tr | et | fi | hu |    |
|-----------------|----|----|----|----|----|----|----|----|----|----|----|----|----|----|----|----|----|----|----|----|----|----|----|----|----|----|----|----|----|----|----|----|----|----|----|----|----|----|----|----|----|
| ar              |    | 3  | 5  | 0  | 22 | 10 | 14 | 20 | 28 | 3  | 51 | 17 | 50 | 34 | 25 | 5  | 55 | 0  | 25 | 17 | 4  | 16 | 12 | 15 | 6  | 50 | 10 | 33 | 15 | 7  | 21 | 16 | 38 | 0  | 0  | 32 | 23 | 1  | 10 | 13 | 12 |
| he              | 36 |    | 12 | 4  | 9  | 21 | 4  | 28 | 29 | 12 | 44 | 24 | 41 | 29 | 32 | 33 | 38 | 19 | 26 | 3  | 45 | 48 | 48 | 36 | 39 | 28 | 38 | 34 | 23 | 12 | 38 | 12 | 42 | 5  | 41 | 38 | 31 | 8  | 34 | 40 | 33 |
| id              | 8  | 28 |    | 63 | 35 | 49 | 45 | 34 | 52 | 51 | 44 | 64 | 72 | 53 | 44 | 36 | 5  | 0  | 3  | 0  | 48 | 46 | 52 | 78 | 44 | 48 | 28 | 24 | 24 | 28 | 50 | 63 | 50 | 73 | 60 | 61 | 35 | 41 | 59 | 46 | 50 |
| ms              | 4  | 23 | 73 |    | 54 | 65 | 55 | 38 | 62 | 65 | 59 | 65 | 70 | 66 | 57 | 26 | 5  | 0  | 2  | 0  | 65 | 64 | 71 | 72 | 63 | 64 | 20 | 18 | 24 | 27 | 58 | 68 | 59 | 71 | 57 | 66 | 37 | 61 | 44 | 42 | 60 |
| tl              | 3  | 20 | 64 | 54 |    | 66 | 36 | 41 | 39 | 54 | 45 | 74 | 45 | 44 | 47 | 31 | 2  | 0  | 2  | 0  | 61 | 67 | 61 | 57 | 47 | 69 | 27 | 27 | 28 | 30 | 51 | 54 | 54 | 57 | 51 | 58 | 40 | 58 | 40 | 48 | 32 |
| vi              | 4  | 18 | 50 | 47 | 33 |    | 36 | 31 | 33 | 42 | 41 | 52 | 42 | 40 | 39 | 26 | 3  | 0  | 2  | 0  | 54 | 53 | 53 | 51 | 49 | 51 | 23 | 18 | 21 | 24 | 41 | 46 | 48 | 48 | 45 | 45 | 32 | 44 | 38 | 42 | 41 |
| it              | 12 | 31 | 66 | 59 | 42 | 57 |    | 70 | 62 | 71 | 60 | 60 | 73 | 74 | 54 | 38 | 6  | 0  | 5  | 1  | 65 | 67 | 68 | 71 | 69 | 67 | 40 | 41 | 38 | 44 | 70 | 74 | 74 | 73 | 71 | 70 | 57 | 68 | 71 | 71 | 69 |
| lv              | 12 | 29 | 59 | 54 | 49 | 53 | 64 |    | 52 | 64 | 51 | 61 | 64 | 63 | 44 | 29 | 6  | 0  | 9  | 2  | 57 | 64 | 61 | 63 | 62 | 62 | 32 | 35 | 30 | 35 | 62 | 63 | 65 | 63 | 66 | 62 | 53 | 59 | 65 | 65 | 61 |
| af              | 10 | 23 | 69 | 59 | 38 | 52 | 63 | 56 |    | 74 | 66 | 68 | 79 | 72 | 57 | 42 | 4  | 0  | 7  | 0  | 55 | 61 | 68 | 74 | 55 | 66 | 31 | 37 | 33 | 37 | 68 | 71 | 68 | 73 | 66 | 62 | 54 | 60 | 67 | 72 | 70 |
| da              | 10 | 35 | 72 | 65 | 47 | 60 | 68 | 65 | 65 |    | 67 | 74 | 79 | 80 | 62 | 43 | 5  | 0  | 6  | 0  | 72 | 73 | 74 | 76 | 72 | 71 | 41 | 43 | 45 | 39 | 68 | 76 | 75 | 77 | 75 | 72 | 59 | 71 | 73 | 74 | 73 |
| de              | 8  | 28 | 57 | 53 | 37 | 49 | 56 | 54 | 57 | 66 |    | 61 | 69 | 66 | 55 | 35 | 7  | 0  | 7  | 0  | 55 | 58 | 61 | 65 | 54 | 56 | 29 | 34 | 39 | 32 | 58 | 65 | 60 | 65 | 62 | 58 | 49 | 63 | 62 | 59 | 61 |
| en              | 5  | 21 | 58 | 52 | 45 | 56 | 44 | 44 | 44 | 58 | 52 |    | 60 | 52 | 45 | 33 | 4  | 0  | 4  | 0  | 58 | 60 | 57 | 59 | 57 | 55 | 27 | 28 | 33 | 33 | 49 | 55 | 55 | 58 | 53 | 51 | 38 | 58 | 48 | 53 | 52 |
| no              | 12 | 33 | 68 | 60 | 46 | 59 | 60 | 60 | 64 | 76 | 70 | 72 |    | 76 | 60 | 39 | 8  | 0  | 7  | 1  | 68 | 70 | 73 | 79 | 69 | 71 | 40 | 38 | 38 | 39 | 65 | 75 | 71 | 77 | 70 | 69 | 54 | 70 | 67 | 71 | 70 |
| sv              | 11 | 33 | 69 | 55 | 41 | 52 | 67 | 57 | 68 | 74 | 70 | 69 | 78 |    | 62 | 46 | 6  | 0  | 6  | 0  | 62 | 72 | 76 | 77 | 73 | 72 | 38 | 42 | 47 | 41 | 70 | 72 | 75 | 78 | 66 | 72 | 59 | 69 | 71 | 68 | 69 |
| el              | 21 | 32 | 60 | 56 | 29 | 47 | 65 | 62 | 63 | 77 | 73 | 63 | 76 | 84 |    | 41 | 10 | 0  | 4  | 0  | 63 | 62 | 66 | 61 | 63 | 69 | 33 | 39 | 40 | 48 | 64 | 61 | 65 | 61 | 66 | 66 | 55 | 67 | 68 | 71 | 64 |
| fa              | 39 | 24 | 28 | 35 | 23 | 7  | 14 | 12 | 5  | 9  | 22 | 15 | 9  | 19 | 22 |    | 41 | 15 | 27 | 28 | 29 | 30 | 44 | 8  | 28 | 25 | 9  | 7  | 8  | 8  | 20 | 30 | 11 | 7  | 37 | 8  | 20 | 12 | 8  | 27 | 15 |
| fr              | 22 | 3  | 4  | 2  | 22 | 11 | 14 | 20 | 25 | 2  | 59 | 7  | 48 | 32 | 36 | 1  |    | 0  | 27 | 26 | 6  | 22 | 24 | 11 | 6  | 48 | 5  | 25 | 23 | 8  | 23 | 9  | 34 | 2  | 0  | 35 | 37 | 0  | 7  | 20 | 24 |
| bn              | 61 | 56 | 47 | 51 | 54 | 55 | 40 | 32 | 41 | 56 | 52 | 43 | 24 | 40 | 43 | 42 | 53 |    | 55 | 52 | 58 | 52 | 59 | 54 | 56 | 44 | 21 | 34 | 37 | 51 | 36 | 41 | 47 | 47 | 44 | 51 | 31 | 38 | 50 | 53 | 47 |
| hi              | 51 | 47 | 51 | 49 | 45 | 35 | 20 | 28 | 19 | 45 | 36 | 21 | 38 | 26 | 33 | 3  | 52 | 45 |    | 10 | 41 | 46 | 45 | 36 | 52 | 37 | 25 | 28 | 17 | 36 | 27 | 36 | 37 | 27 | 30 | 41 | 20 | 35 | 30 | 20 | 32 |
| ta              | 38 | 32 | 24 | 7  | 23 | 18 | 17 | 19 | 16 | 23 | 29 | 16 | 24 | 17 | 18 | 20 | 31 | 31 | 7  |    | 27 | 29 | 26 | 25 | 33 | 23 | 22 | 21 | 22 | 23 | 17 | 23 | 27 | 24 | 25 | 24 | 15 | 23 | 20 | 26 | 28 |
| ca              | 6  | 24 | 68 | 63 | 57 | 69 | 56 | 56 | 54 | 72 | 67 | 76 | 78 | 68 | 56 | 36 | 5  | 0  | 4  | 0  |    | 81 | 82 | 81 | 81 | 76 | 37 | 35 | 37 | 43 | 60 | 69 | 68 | 76 | 67 | 63 | 50 | 67 | 63 | 68 | 67 |
| es              | 6  | 26 | 68 | 50 | 45 | 54 | 58 | 42 | 59 | 63 | 70 | 64 | 80 | 74 | 61 | 43 | 6  | 0  | 5  | 0  | 63 |    | 83 | 81 | 84 | 78 | 32 | 38 | 41 | 48 | 57 | 71 | 74 | 77 | 57 | 69 | 56 | 64 | 56 | 58 | 56 |
| fr              | 6  | 25 | 63 | 58 | 45 | 61 | 55 | 49 | 55 | 68 | 63 | 71 | 78 | 73 | 54 | 36 | 4  | 0  | 5  | 0  | 72 | 79 |    | 80 | 77 | 74 | 27 | 32 | 33 | 39 | 56 | 72 | 69 | 74 | 65 | 64 | 50 | 61 | 58 | 65 | 64 |
| it              | 12 | 31 | 67 | 63 | 48 | 64 | 58 | 58 | 57 | 74 | 64 | 73 | 77 | 73 | 53 | 36 | 9  | 0  | 6  | 0  | 74 | 72 | 78 |    | 72 | 69 | 36 | 39 | 38 | 44 | 64 | 75 | 70 | 77 | 70 | 67 | 56 | 68 | 64 | 70 | 70 |
| pt              | 7  | 28 | 60 | 56 | 47 | 58 | 55 | 48 | 51 | 69 | 66 | 68 | 74 | 70 | 54 | 38 | 6  | 0  | 4  | 0  | 71 | 81 | 79 | 78 |    | 73 | 32 | 36 | 37 | 40 | 55 | 70 | 68 | 74 | 63 | 62 | 52 | 64 | 58 | 67 | 62 |
| ro              | 6  | 24 | 65 | 52 | 44 | 59 | 50 | 38 | 64 | 59 | 64 | 57 | 72 | 70 | 61 | 38 | 4  | 0  | 3  | 0  | 56 | 77 | 70 | 73 | 74 |    | 26 | 35 | 28 | 41 | 54 | 60 | 71 | 58 | 52 | 65 | 50 | 51 | 43 | 57 | 42 |
| bg              | 26 | 13 | 19 | 6  | 10 | 4  | 4  | 4  | 6  | 15 | 35 | 3  | 5  | 8  | 25 | 5  | 39 | 21 | 18 | 27 | 15 | 20 | 7  | 4  | 28 | 17 |    | 73 | 76 | 73 | 8  | 4  | 4  | 11 | 4  | 4  | 4  | 10 | 5  | 5  | 13 |
| mk              | 17 | 7  | 9  | 3  | 7  | 12 | 12 | 2  | 6  | 10 | 36 | 2  | 3  | 5  | 28 | 3  | 35 | 17 | 14 | 21 | 8  | 13 | 4  | 2  | 15 | 10 | 72 |    | 63 | 72 | 15 | 2  | 2  | 7  | 2  | 3  | 2  | 6  | 4  | 3  | 7  |
| ru              | 12 | 13 | 16 | 9  | 9  | 8  | 7  | 8  | 8  | 14 | 29 | 7  | 9  | 10 | 19 | 10 | 25 | 17 | 13 | 16 | 14 | 20 | 10 | 9  | 18 | 14 | 52 | 39 |    | 61 | 10 | 10 | 7  | 11 | 9  | 9  | 9  | 13 | 10 | 9  | 12 |
| uk              | 17 | 11 | 14 | 9  | 7  | 4  | 5  | 5  | 5  | 11 | 27 | 3  | 4  | 6  | 21 | 6  | 33 | 19 | 17 | 25 | 14 | 14 | 7  | 5  | 19 | 16 | 56 | 58 | 60 |    | 6  | 12 | 4  | 10 | 5  | 5  | 5  | 8  | 7  | 12 | 9  |
| bs              | 9  | 23 | 62 | 50 | 37 | 47 | 62 | 56 | 57 | 66 | 63 | 58 | 70 | 67 | 55 | 33 | 6  | 1  | 4  | 0  | 58 | 66 | 63 | 69 | 62 | 66 | 31 | 35 | 31 | 41 |    | 72 | 80 | 71 | 69 | 67 | 52 | 56 | 61 | 67 | 61 |
| cs              | 12 | 35 | 64 | 59 | 40 | 56 | 60 | 58 | 54 | 68 | 62 | 67 | 71 | 70 | 52 | 41 | 7  | 0  | 8  | 1  | 64 | 70 | 70 | 72 | 67 | 65 | 39 | 41 | 39 | 40 | 65 |    | 73 | 75 | 77 | 70 | 56 | 63 | 63 | 68 | 67 |
| hr              | 10 | 31 | 64 | 52 | 39 | 52 | 65 | 59 | 58 | 71 | 60 | 63 | 72 | 71 | 53 | 40 | 5  | 0  | 6  | 1  | 63 | 70 | 68 | 72 | 68 | 68 | 38 | 39 | 38 | 38 | 75 | 77 |    | 74 | 74 | 73 | 58 | 64 | 65 | 71 | 69 |
| pl              | 11 | 33 | 68 | 64 | 43 | 58 | 60 | 59 | 63 | 74 | 65 | 69 | 76 | 75 | 51 | 44 | 8  | 0  | 7  | 1  | 70 | 69 | 72 | 77 | 70 | 70 | 40 | 36 | 43 | 42 | 71 | 78 | 73 |    | 75 | 69 | 52 | 70 | 69 | 71 | 73 |
| sk              | 11 | 34 | 62 | 58 | 39 | 55 | 62 | 61 | 56 | 69 | 67 | 64 | 75 | 69 | 55 | 39 | 12 | 0  | 6  | 1  | 70 | 74 | 68 | 74 | 72 | 67 | 38 | 38 | 37 | 37 | 67 | 79 | 70 | 73 |    | 67 | 56 | 63 | 67 | 68 | 69 |
| sl              | 14 | 34 | 66 | 63 | 49 | 58 | 65 | 61 | 64 | 69 | 59 | 67 | 73 | 70 | 56 | 38 | 11 | 1  | 7  | 1  | 66 | 73 | 74 | 75 | 71 | 73 | 37 | 40 | 42 | 45 | 67 | 73 | 77 | 72 | 72 |    | 57 | 65 | 65 | 70 | 68 |
| sq              | 20 | 42 | 77 | 70 | 58 | 69 | 73 | 64 |    |    |    |    |    |    |    |    |    |    |    |    |    |    |    |    |    |    |    |    |    |    |    |    |    |    |    |    |    |    |    |    |    |

|            |           |           | Supervised |      |         |          |          |                                       |                     | Unsupervised |                                       |                                   |                                   |                   |        |      |
|------------|-----------|-----------|------------|------|---------|----------|----------|---------------------------------------|---------------------|--------------|---------------------------------------|-----------------------------------|-----------------------------------|-------------------|--------|------|
| #train (k) | #test (k) | BiDic.P@1 | HSup       | LSup | RaRe t1 | RaRe t10 | RaRe all | BEA <sub>sup</sub> <sup>ent</sup> t10 | RaRe <sub>uns</sub> | BWET         | BEA <sub>uns</sub> <sup>ent</sup> t10 | BEA <sub>uns</sub> <sup>ent</sup> | BEA <sub>uns</sub> <sup>tok</sup> | MV <sup>tok</sup> | Oracle |      |
|            |           |           |            |      |         |          |          |                                       |                     |              |                                       |                                   |                                   |                   |        |      |
| af         | 5         | 1         | 36         | 84   | 59      | 73       | 79       | 79                                    | 80                  | 76           | 64                                    | 79                                | 79                                | 74                | 75     | 80   |
| ar         | 20        | 10        | 46         | 88   | 64      | 71       | 74       | 74                                    | 65                  | 26           | 19                                    | 54                                | 45                                | 54                | 12     | 56   |
| bg         | 20        | 10        | 55         | 90   | 61      | 80       | 81       | 81                                    | 81                  | 5            | 51                                    | 81                                | 65                                | 54                | 4      | 76   |
| bn         | 10        | 1         | 1          | 95   | 70      | 68       | 74       | 74                                    | 69                  | 65           | 36                                    | 67                                | 66                                | 60                | 56     | 63   |
| bs         | 15        | 1         | 30         | 92   | 63      | 80       | 79       | 80                                    | 78                  | 76           | 52                                    | 80                                | 78                                | 77                | 69     | 82   |
| ca         | 20        | 10        | 70         | 91   | 62      | 82       | 86       | 84                                    | 86                  | 80           | 62                                    | 85                                | 80                                | 79                | 72     | 83   |
| cs         | 20        | 10        | 64         | 90   | 62      | 77       | 78       | 75                                    | 78                  | 73           | 59                                    | 77                                | 75                                | 72                | 71     | 78   |
| da         | 20        | 10        | 68         | 90   | 62      | 77       | 81       | 81                                    | 82                  | 79           | 68                                    | 83                                | 82                                | 79                | 78     | 80   |
| de         | 20        | 10        | 73         | 86   | 58      | 73       | 74       | 73                                    | 72                  | 69           | 63                                    | 72                                | 71                                | 64                | 68     | 70   |
| el         | 20        | 10        | 55         | 89   | 61      | 67       | 67       | 67                                    | 54                  | 13           | 45                                    | 49                                | 43                                | 34                | 13     | 45   |
| en         | 20        | 10        | —          | 81   | 47      | 64       | 65       | 64                                    | 65                  | 58           | —                                     | 63                                | 61                                | 57                | 56     | 61   |
| es         | 20        | 10        | 83         | 90   | 63      | 83       | 84       | 84                                    | 85                  | 76           | 62                                    | 85                                | 81                                | 76                | 73     | 84   |
| et         | 15        | 10        | 41         | 90   | 64      | 73       | 77       | 77                                    | 78                  | 72           | 58                                    | 78                                | 78                                | 71                | 73     | 75   |
| fa         | 20        | 10        | 33         | 93   | 74      | 78       | 81       | 79                                    | 69                  | 30           | 16                                    | 65                                | 50                                | 52                | 15     | 60   |
| fi         | 20        | 10        | 58         | 89   | 67      | 78       | 80       | 80                                    | 81                  | 76           | 68                                    | 81                                | 80                                | 69                | 77     | 78   |
| fr         | 20        | 10        | 82         | 88   | 57      | 81       | 81       | 80                                    | 84                  | 75           | 59                                    | 83                                | 79                                | 73                | 71     | 80   |
| he         | 20        | 10        | 52         | 85   | 53      | 61       | 61       | 60                                    | 55                  | 40           | 26                                    | 54                                | 54                                | 46                | 34     | 50   |
| hi         | 5         | 1         | 29         | 85   | 68      | 64       | 74       | 73                                    | 68                  | 48           | 27                                    | 64                                | 61                                | 58                | 35     | 54   |
| hr         | 20        | 10        | 48         | 89   | 61      | 74       | 79       | 78                                    | 80                  | 76           | 49                                    | 80                                | 79                                | 77                | 73     | 78   |
| hu         | 20        | 10        | 64         | 90   | 59      | 75       | 79       | 78                                    | 80                  | 71           | 55                                    | 79                                | 79                                | 69                | 73     | 76   |
| id         | 20        | 10        | 68         | 91   | 67      | 82       | 83       | 81                                    | 75                  | 59           | 62                                    | 73                                | 67                                | 61                | 62     | 79   |
| it         | 20        | 10        | 77         | 89   | 60      | 80       | 81       | 80                                    | 82                  | 75           | 59                                    | 81                                | 78                                | 76                | 72     | 79   |
| lt         | 10        | 10        | 26         | 86   | 62      | 72       | 79       | 80                                    | 79                  | 76           | 48                                    | 80                                | 80                                | 75                | 77     | 74   |
| lv         | 10        | 10        | 31         | 91   | 68      | 70       | 75       | 75                                    | 69                  | 68           | 40                                    | 69                                | 69                                | 67                | 65     | 66   |
| mk         | 10        | 1         | 50         | 91   | 67      | 79       | 82       | 81                                    | 80                  | 4            | 38                                    | 79                                | 66                                | 48                | 3      | 75   |
| ms         | 20        | 1         | 48         | 91   | 66      | 78       | 80       | 78                                    | 74                  | 69           | 62                                    | 68                                | 67                                | 63                | 68     | 74   |
| nl         | 20        | 10        | 76         | 89   | 59      | 78       | 80       | 80                                    | 81                  | 77           | 63                                    | 82                                | 81                                | 78                | 76     | 79   |
| no         | 20        | 10        | 67         | 90   | 65      | 79       | 82       | 81                                    | 83                  | 79           | 59                                    | 83                                | 83                                | 77                | 79     | 79   |
| pl         | 20        | 10        | 66         | 89   | 61      | 76       | 79       | 78                                    | 81                  | 73           | 63                                    | 82                                | 80                                | 77                | 76     | 78   |
| pt         | 20        | 10        | 80         | 90   | 59      | 79       | 81       | 80                                    | 82                  | 77           | 65                                    | 82                                | 77                                | 74                | 70     | 82   |
| ro         | 20        | 10        | 67         | 92   | 66      | 80       | 82       | 82                                    | 80                  | 76           | 46                                    | 78                                | 76                                | 74                | 67     | 77   |
| ru         | 20        | 10        | 59         | 86   | 53      | 73       | 71       | 71                                    | 56                  | 10           | 38                                    | 53                                | 40                                | 36                | 11     | 61   |
| sk         | 20        | 10        | 52         | 91   | 62      | 76       | 79       | 79                                    | 80                  | 74           | 50                                    | 79                                | 76                                | 76                | 71     | 79   |
| sl         | 15        | 10        | 47         | 92   | 64      | 76       | 80       | 80                                    | 79                  | 76           | 58                                    | 79                                | 78                                | 76                | 73     | 78   |
| sq         | 5         | 1         | 37         | 88   | 69      | 79       | 84       | 84                                    | 83                  | 82           | 59                                    | 83                                | 84                                | 76                | 79     | 79   |
| sv         | 20        | 10        | 61         | 93   | 69      | 83       | 83       | 84                                    | 82                  | 77           | 60                                    | 79                                | 80                                | 69                | 76     | 84   |
| ta         | 15        | 1         | 7          | 84   | 54      | 44       | 53       | 53                                    | 46                  | 35           | 12                                    | 39                                | 42                                | 25                | 29     | 38   |
| tl         | 10        | 1         | 20         | 93   | 66      | 75       | 82       | 80                                    | 78                  | 65           | 60                                    | 62                                | 60                                | 57                | 52     | 76   |
| tr         | 20        | 10        | 61         | 90   | 61      | 75       | 77       | 77                                    | 77                  | 70           | 53                                    | 77                                | 76                                | 67                | 67     | 71   |
| uk         | 20        | 10        | 45         | 89   | 60      | 70       | 78       | 79                                    | 70                  | 5            | 35                                    | 64                                | 58                                | 49                | 6      | 60   |
| vi         | 20        | 10        | 54         | 88   | 55      | 64       | 72       | 72                                    | 61                  | 58           | 53                                    | 56                                | 55                                | 48                | 47     | 56   |
| $\mu$      | —         | —         | —          | 89.2 | 62.1    | 74.3     | 77.4     | 76.9                                  | 74.8                | 60.2         | 50.5                                  | 72.8                              | 69.7                              | 64.5              | 56.7   | 71.6 |
| $\sigma$   | —         | —         | —          | 2.8  | 5.2     | 7.3      | 6.4      | 6.4                                   | 9.6                 | 24.1         | 14.7                                  | 11.5                              | 12.6                              | 13.7              | 25     | 11.5 |

**Table 4:** The size of training and test sets (development set size equals test set size) in thousand sentences, and the precision at 1 for Bilingual dictionaries induced from mapping languages to the English embedding space (using identical characters) is shown (BiDic.P@1). F<sub>1</sub> scores on the test set, comparing baseline supervised models (HSup, LSup), multilingual transfer from top  $k$  source languages (RaRe, 5 runs,  $k = 1, 10, 40$ ), an unsupervised RaRe with uniform expertise and no fine-tuning (RaRe<sub>uns</sub>), and aggregation methods: majority voting (MV<sup>tok</sup>), BEA<sub>uns</sub><sup>tok</sup> and BEA<sub>uns</sub><sup>ent</sup> (Bayesian aggregation in token- and entity-level), and the oracle single best annotation (Oracle). We also compare with BWET (Xie et al., 2018), an unsupervised transfer model with state-of-the-art on CoNLL NER datasets. The mean and standard deviation over all 41 languages,  $\mu$ ,  $\sigma$ , are also reported.
